# Supplementary material for: Augmented Electronic Ising Machine as an Effective SAT Solver
Source: arXiv:2305.01623 source file (2023-05-01)
Supplement: Supplementary file 2 [file 7appendix.tex]

\begin{appendices}

\section{Quadratic penalty}
\label{app:kzfd}

The Rosenberg formulation~\cite{rosen} is fairly easy to understand. Given that
we want to replace $x_1x_2$ by $z$, the original cubic term $\pm x_1x_2x_3$ 
is replaced by $\pm zx_3+k\cdot p(x_1, x_2, x_3, z)$, where $p(\cdot )$ 
has to be a quadratic function, expressed as:
\begin{equation}
    \begin{split}
        p(x_1, x_2, x_3, z) & = ax_1x_2 + b(x_1+x_2)x_3 + c (x_1+x_2)z \\ 
        & + d (x_1+x_2) +  ex_3 +  fz 
    \end{split}
\end{equation}
Here due to symmetry, $x_1$ and $x_2$ always have the same coefficient.
To keep the substitution difference 0 when $z=x_1x_2$ we get the following constraints
based on the tuple $(x_1, x_2, z)$
\begin{equation}
    \begin{split}
       (0, 0, 0)&: e=0 \\
       (0, 1, 0), (1, 0, 0)&: \forall x_3, bx_3+d =0 \rightarrow b, d = 0 \\
       (1, 1, 1)&: a +  2c + f = 0 \rightarrow c=-\frac{a+f}{2}.
    \end{split}
\end{equation}
Thus $p(\cdot)$ can be simplified as:
\begin{equation}
p(x_1, x_2, x_3 ,z) = a\cdot x_1x_2 -\frac{a+f}{2}(x_1+x_2)z+f\cdot z
\label{eq:after_eq_constraints}
\end{equation}
When $z\neq x_1x_2$, we need the difference before and after substitution
to be greater than 0. 
\begin{equation}
    \forall z\neq x_1x_2, \pm (zx_3-x_1x_2x_3)+k\cdot p(x_1, x_2, x_3 ,z) > 0
\end{equation}
These constraints can be again separated based on tuple $(x_1, x_2, z)$:
\begin{equation}
    \begin{split}
       (0, 0, 1)&: \forall x_3, kf\pm x_3 > 0 \rightarrow kf>1 \\
       (0, 1, 1), (1, 0, 1)&: \forall x_3, k\frac{f-a}{2} \pm x_3 > 0 \rightarrow k(f-a)>2\\
       (1, 1, 0)&: ka\mp x_3 > 0 \rightarrow ka>1 
    \end{split}
\end{equation}
It is not hard to see that if we assume $k>1$, then an integer solution would
be $a=1; c=2; f=3$, this leads to:
\begin{equation}
p(x_1, x_2, z) = x_1x_2 -2(x_1+x_2)z+3z
\end{equation}

We can improve upon this substitution. Consider a simple Hamiltonian
$ -x_1x_2x_3$ which has 8 phase points, with 
the ground state $(x_1,x_2,x_3)=(1,1,1)$ representing 1/8 of the entire phase space volume.
After substitution, the landscape has 16 phase points, with the ground state
$(x_1,x_2,x_3,z)=(1,1,1,1)$ representing 1/16 of the entire phase space volume, and thus
harder to reach. If we change our strategy and not penalize the phase point $(1,1,1,0)$
we can increase the chance of finding the ground state. In other words, when $z\neq x_1x_2$,
we no longer require substitution difference to be (strictly) greater than 0, other that
it is non-negative. Eq.~\ref{eq:after_eq_constraints} still holds. We update the case
$z\neq x_1x_2$. Furthermore, we handle the substitution of $\pm x_1x_2x_3$ separately.

For the positive term, the difference will be \begin{equation}
-x_1x_2x_3 + x_3z + ax_1x_2 -\frac{a+f}{2}(x_1+x_2)z+fz \ge 0.
\end{equation}
Based on the tuple $(x_1, x_2, z)$, the constraints become: 
\begin{equation}
    \begin{split}
        (0, 0, 1)&: x_3 + f \ge 0 \rightarrow f\ge 0; \\
        (0, 1, 1), (1, 0, 1)&:  x_3-(a+f)/2+f \ge 0; \rightarrow f\ge a; \\
        (1, 1, 0)&: -x_3 + a \ge 0 \rightarrow a \ge 1.
    \end{split}
\end{equation}
It is not hard to see $a=f=1$ satisfies the constraints. 

For the negative term, the difference will be \begin{equation}
+x_1x_2x_3 - x_3z + ax_1x_2 -\frac{a+f}{2}(x_1+x_2)z+fz \ge 0.
\end{equation}
Based on the tuple $(x_1, x_2, z)$, the constraints become: 
\begin{equation}
    \begin{split}
        (0, 0, 1)&: -x_3 + f \ge 0 \rightarrow f\ge 1; \\
        (0, 1, 1), (1, 0, 1)&: -x_3+(f-a)/2 \ge 0; \rightarrow f\ge a+2; \\
        (1, 1, 0)&:  x_3 + a \ge 0 \rightarrow a \ge 0.
    \end{split}
\end{equation}
It is not hard to see $a=0, f=2$ satisfies the constraints. 
This leads to the KZFD rule shown in Eq.~\ref{eq:kzfd}.

\section{QAOA}
\label{app:qaoa}

QAOA   circuit consists of two operators, repeated a preset number of times $p$. Each operator corresponds to time evolution of a particular Hamiltonian. Suppose we have defined some cost function $C$ which we wish to minimize for an $N$-variable quadratic problem. We now define:
\begin{equation}
        B=\sum_{j=1}^NX_j
\end{equation}
where $X_j$ is the unitary Pauli $X$ operator acting on the $j^{th}$ qubit. We then define two operators:
\begin{equation}
    \begin{split}
        U_B(\beta)&=e^{-i\beta B}=\prod_{j=1}^Ne^{\beta X_j}\\
        U_C(\gamma)&=e^{-i\gamma C}
    \end{split}
\end{equation}
For a given $p$ value and initial state $\ket{s_0}$, the QAOA circuit can then be represented as:
\begin{equation}
    \ket{\bm{\gamma}, \bm{\beta}} = U_B(\beta_p)U_C(\gamma_p)...U_B(\beta_1)U_C(\gamma_1)\ket{s_0}
\end{equation}
This circuit has $2p$ parameters, often referred to as "angles". If we define the resulting state $F_p(\gamma, \beta)$ of the circuit as the expectation value of $C$:
\begin{equation}
    F_p(\bm{\gamma}, \bm{\beta})=\expval{C}{\bm{\gamma}, \bm{\beta}}
\end{equation}
then it has been shown \cite{qaoa_original} there exist angles $\bm{\gamma^*}, \bm{\beta^*}$ such that in the limit as $p\to \infty$:
\begin{equation}
    F_p(\bm{\gamma^*}, \bm{\beta^*})\to C_{\textrm{Min}}
\end{equation}
where $C_{\textrm{Min}}$ is the minimum value of the cost function. However, infinite 
circuit depth is clearly impractical. The theoretical property of fixed $p$ QAOA is uncertain.
Taking into account gate errors, practical NISQ era QAOA is likely to use $p=1$.

\section{Quantum Analysis Methodology}
\label{appdx:qc_methods}

\subsection{QAOA Simulation}
QAOA was simulated using the Qiskit runtime framework \cite{Qiskit}. Problems were provided as a \texttt{PauliSumOp} object corresponding to a sum of modified clause Hamiltonians defined in \cite{boolean_pauli_hamil} to the \texttt{QAOA} class. The circuits were optimized using the Qiskit implementation of COBYLA, which has been shown to have high performance and solution quality in both noiseless and noisy environments \cite{qaoa_optimizers}. Following previous work in near-term QAOA analysis \cite{qaoa_speedup}, we used 10,000 samples per optimization iteration. At $p=1$, the COBYLA optimizer ran for $\sim$33 iterations. After the simulator output the final state vectors, the sum of the normalized satisfying state amplitudes were used to compute TTS. Simulations of $p=2,4$ were performed as well, with little increase in satisfaction rate. The large increase in optimizer iterations (54 and 92 on average respectively) as well as the detrimental effects of noise on increasing $p$ \cite{qaoa_noise}, motivated the limitation to $p=1$ QAOA for our analysis.
The circuit was constructed using a sum of boolean disjunction Pauli operations defined in \cite{boolean_pauli_hamil}, avoiding QUBO qubit overhead. The solver was computationally limited to fewer than 30 qubits, so circuits were compiled and scheduled for a 127 qubit system for $N=30,\;40$ (Figs. \ref{fig:quantum_comp} \& \ref{fig:brim_sat}) and $N=100$ (Fig. \ref{fig:tts_bench}) with $N=20$ success rates used to extrapolate TTS.

\subsection{QAOA Error Estimation}
We neglect the effects of qubit decoherence/relaxation times on solution quality. For a holistic QAOA noise study, see \cite{qaoa_noise}. Instead, we focus on gate error rates, as effects are estimable for large circuits without simulation or access to high qubit hardware. We wish to quantify the increase in sample count necessary to model the QAOA state distribution. Following the methodology in \cite{qaoa_noise_shots}, we define the probability of measuring a state from the ideal distribution in the presence of errors as:
\begin{equation}
    F_0=\prod_j(1-\epsilon_j)^{N_j}
\end{equation}
where each $j$ denotes distinct gate types. $N_j$ corresponds to the number of $j$-type gates, and $\epsilon_j$ to the associated error probability. This consisted of coupled \emph{CX} and unitary $\sqrt{X}$ and $\textrm{Pauli}\;X$ gates for the \emph{ibmq\_washington} system \cite{ibm_quantum}. The error rates for coupled and unitary gates were $1.203\times 10^{-2}$ and $3.006\times 10^{-4}$ respectively: taken from recent IBM calibration data \cite{ibm_quantum}. From this $F_0$, we bound the sample count $M$ needed to produce a single sample from the ideal distribution with probability $P$ as:
\begin{equation}
    M\leq\frac{\log_{10}(1-P)}{\log_{10}(1-F_0)}
\end{equation}
For our analysis, $P=0.99$. Since the quality of final QAOA distribution is dependent on the angles determined by the optimizer, errors motivate increases in the sample count for both the optimizer iterations as well as the final circuit query. Hence, $M$ is treated as a scaling factor for the \emph{total} number of samples needed, reflected in Fig. \ref{fig:quantum_comp}.

The Qiskit QAOA circuits used for this analysis were constructed from \texttt{PauliSumOp} objects using the \texttt{QAOAAnsatz} circuit class and transpiled for the \emph{ibmq\_washington} system ~\cite{Qiskit, ibm_quantum}. The circuit analysis then accounts for the additional coupled gates introduced by IBM's hex-heavy topology \cite{qaoa_sabre}, though SABRE routing and layout heuristics were used to reduce high-error coupling gates ~\cite{sabre, qaoa_sabre}. 
\subsection{QA Sampling}
\begin{table}[!ht]\centering
    \caption{Annealing times used for QA sampling}
    \begin{tabular}{|c|c|}
    \hline
        \textbf{Vars} & \textbf{Anneal ($\mu s$)} \\\hline\hline
        5-7 & 2\\\hline
        8,10,20 & 20\\\hline
        30,40 & 2000\\\hline
    \end{tabular}
    % \hfill
    \label{tab:qa_anneal}
\end{table}
The D-Wave 2000Q QPU was used for benchmarking the quantum annealing approach. Annealing times varied by problem size: starting with AIMS annealing times as a baseline and increasing as necessary to produce \textit{some} satisfying solutions. Table \ref{tab:qa_anneal} shows the annealing times used. 100 samples were taken per problem for problems of size 5-20. Low success rates necessitated 400 samples for the 30 and 40 variable problems.

\section{Circuit}\label{app:circuit}

A circuit-based implementation has been developed in Cadence and simulated with the Virtuoso analog design environment. The overall architecture of the design is discussed in Sec.~\ref{sec:arch}. The design of the  coupling units and nodes of the implementation can be seen in Fig.~\ref{fig:cadence_coupling_unit} and Fig.~\ref{fig:cadence_node}, respectively. 

\begin{figure}[htb]\centering
    \includegraphics[width=0.45\textwidth]{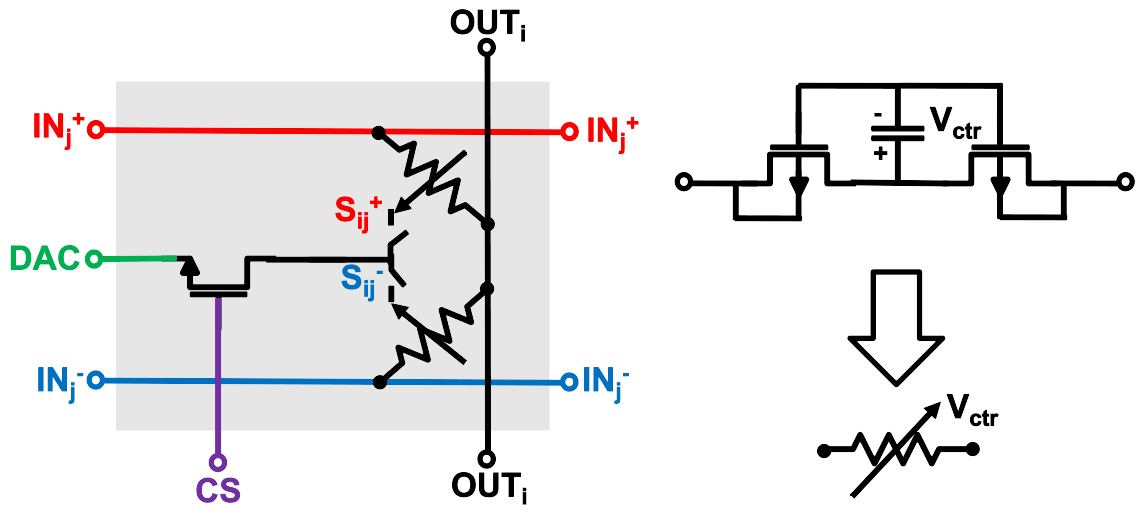}
    \caption{[Left] Architecture of a SAT coupling unit in hardware. [Right] Design of the variable resistor used to program the coupling weights.}
    \label{fig:cadence_coupling_unit}
\end{figure}

The coupling unit includes two programmable resistors and a pair of switches. To enable positive coupling, $S_{ij}^+$ is closed, connecting $OUT_i$  to $IN_j^+$ through a programmable resistor. To enable negative coupling, $S_{ij}^-$ is closed, which connects $OUT_i$ to $IN_j^-$. $S_{ij}^+$ and $S_{ij}^-$ are mutually exclusive, only one can be closed at a time for the circuit to operate as intended.

Implementing resistors directly on-chip is costly in terms of area and does not allow for programmable values to account for different coupling strengths between nodes. To circumvent both of these issues, rather than using a physical resistor, two p-type transistors are connected as displayed in Fig.~\ref{fig:cadence_coupling_unit}, with a capacitor across the source and gate. This configuration has a similar I-V characteristic to a physical resistor while consuming less area, and setting the voltage ($V_{ctr}$) across the capacitor allows for the effective resistance to be tuned, allowing for programmable resistances.

\begin{figure}[htb]\centering
    \includegraphics[width=0.4\textwidth]{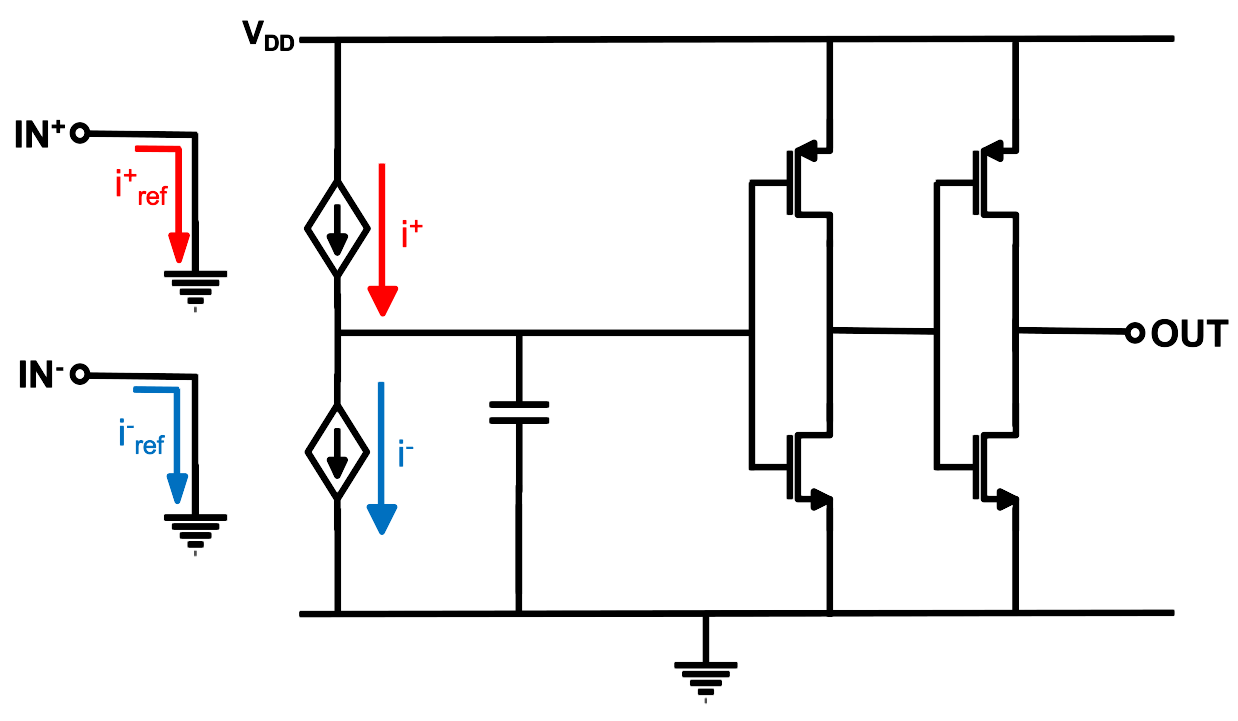}
    \caption{Circuit architecture of a node. The node consists of two current mirrors (left), a capacitor, and a buffer to quantize the voltage (right).}
    \label{fig:cadence_node}
\end{figure}

The node design includes a capacitor, which stores the current state of the node, and a buffer to quantize the output to either $V_{SS}$ or $V_{DD}$. The node takes two current inputs, $IN^+$ and $IN^-$, which are the sum of output currents coming from nodes to which this node is positively and negatively coupled, respectively. The current flowing into $IN^+$ is mirrored to flow from $V_{DD}$ to the positive plate of the capacitor, charging it, and the current flowing into $IN^-$ is mirrored to flow from the positive plate of the capacitor to ground, discharging the capacitor. The net current flowing into the positive plate of the capacitor is $i^+-i^-$, so the result is that if there is greater current flowing into the node from nodes that it is positively coupled to than the incoming current from nodes that it is negatively coupled to, the capacitor will charge, and vice versa.

The Cadence implementation was tested with a fully-connected 6-node graph and all possible inputs were enumerated. The system settled into a local minimum for every possible input, with an average power draw of 200 $\mu W$. Preliminary tests revealed that the power consumption scales with the number of active couplings, rather than the number of nodes, as the resistors in the coupling units dissipate the majority of the energy in the system. Based on this information and an analysis of representative 500-node graphs, we computed as a rough estimate that a 500-node system would be expected to consume, on average, 90 $mW$. The actual power draw is dependent on the number of high nodes (nodes outputting a quantized value of $V_{DD}$) and the number of couplings each high node has, but we are confident in this figure as a high-level, order-of-magnitude estimate.

An initial, course area estimate was also performed using Cadence's layout editor and a 45 $nm$ generic process design kit. Each node measures roughly 8 $\mu m$ $\times$ 9 $\mu m$, and each coupling unit is approximately 1 $\mu m$ $\times$ 1 $\mu m$. The overall chip area will be dominated by the O($N^2$) coupling units. With a chip of, say, 500 variables, the area will be on the orders of $1mm^2$ at 45nm technology. 

%The SAT circuit has been verified in simulation using Cadence and we are continuing to test with larger problems.

\end{appendices}
